# Supplementary material for: Opening the random forest black box by the analysis of the mutual impact of features
Source: arXiv:2304.02490 source file (2023-04-05)
Supplement: Supplementary file 1 [file SupplementaryInformation.pdf]

# Supplementary information “Opening the random forest black box by the analysis of the mutual impact of features”

Lucas F. Voges, Lukas C. Jarren, Stephan Seifert

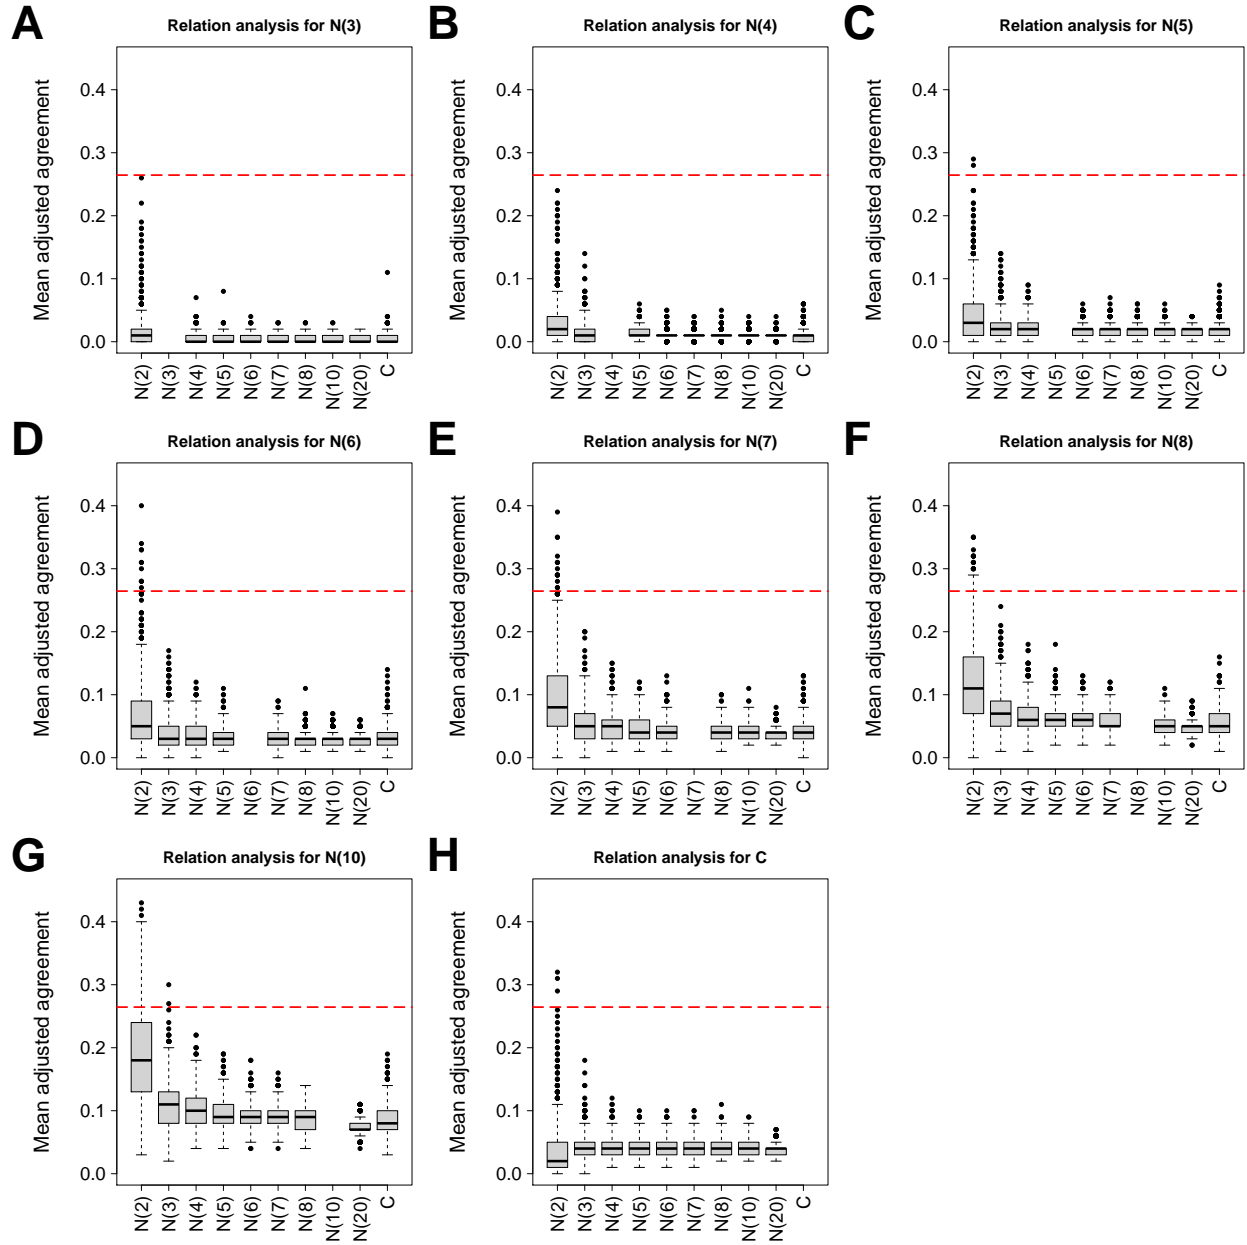

Figure S 1: Null Scenario A (classification): Relation analysis based on mean adjusted agreement for the nominal variables with 3, 4, 5, 6, 7, 8, 10 categories (A-G) and the continuous variable (H). The dashed line shows the threshold for the selection of related variables. The relations of the other variables are shown in Figure 1.

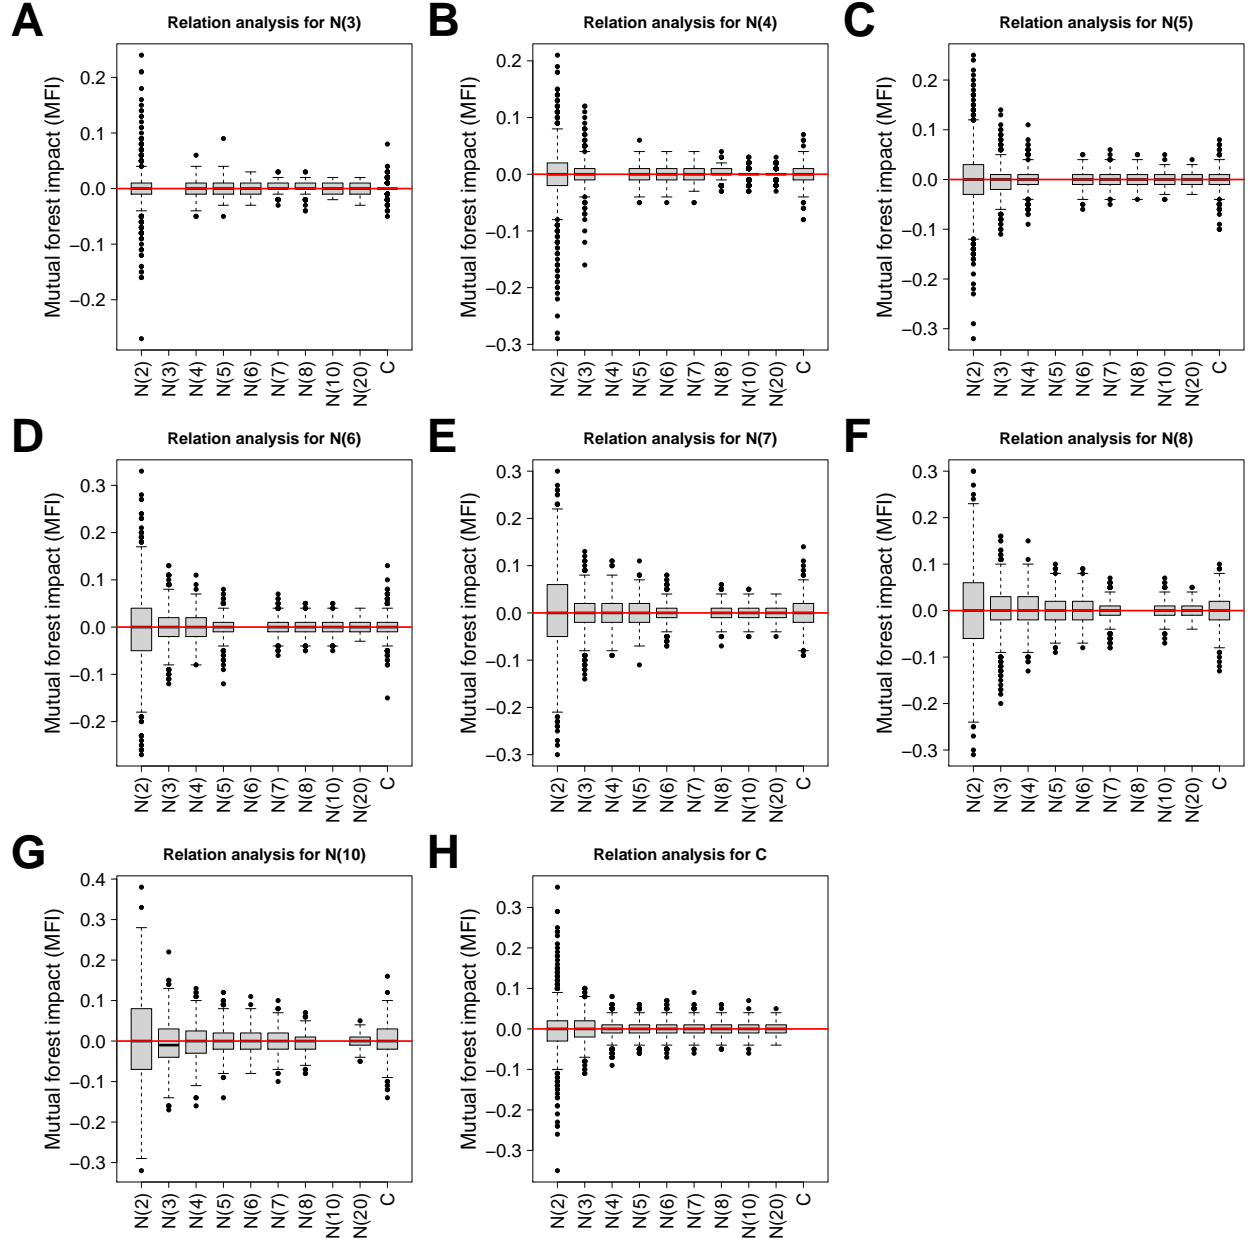

Figure S 2: Null Scenario A (classification): Relation analysis based on MFI for the nominal variables with 3, 4, 5, 6, 7, 8, 10 categories (A-G) and the continuous variable (H). The dashed line shows a relation value of 0. The relations of the other variables are shown in Figure 1.

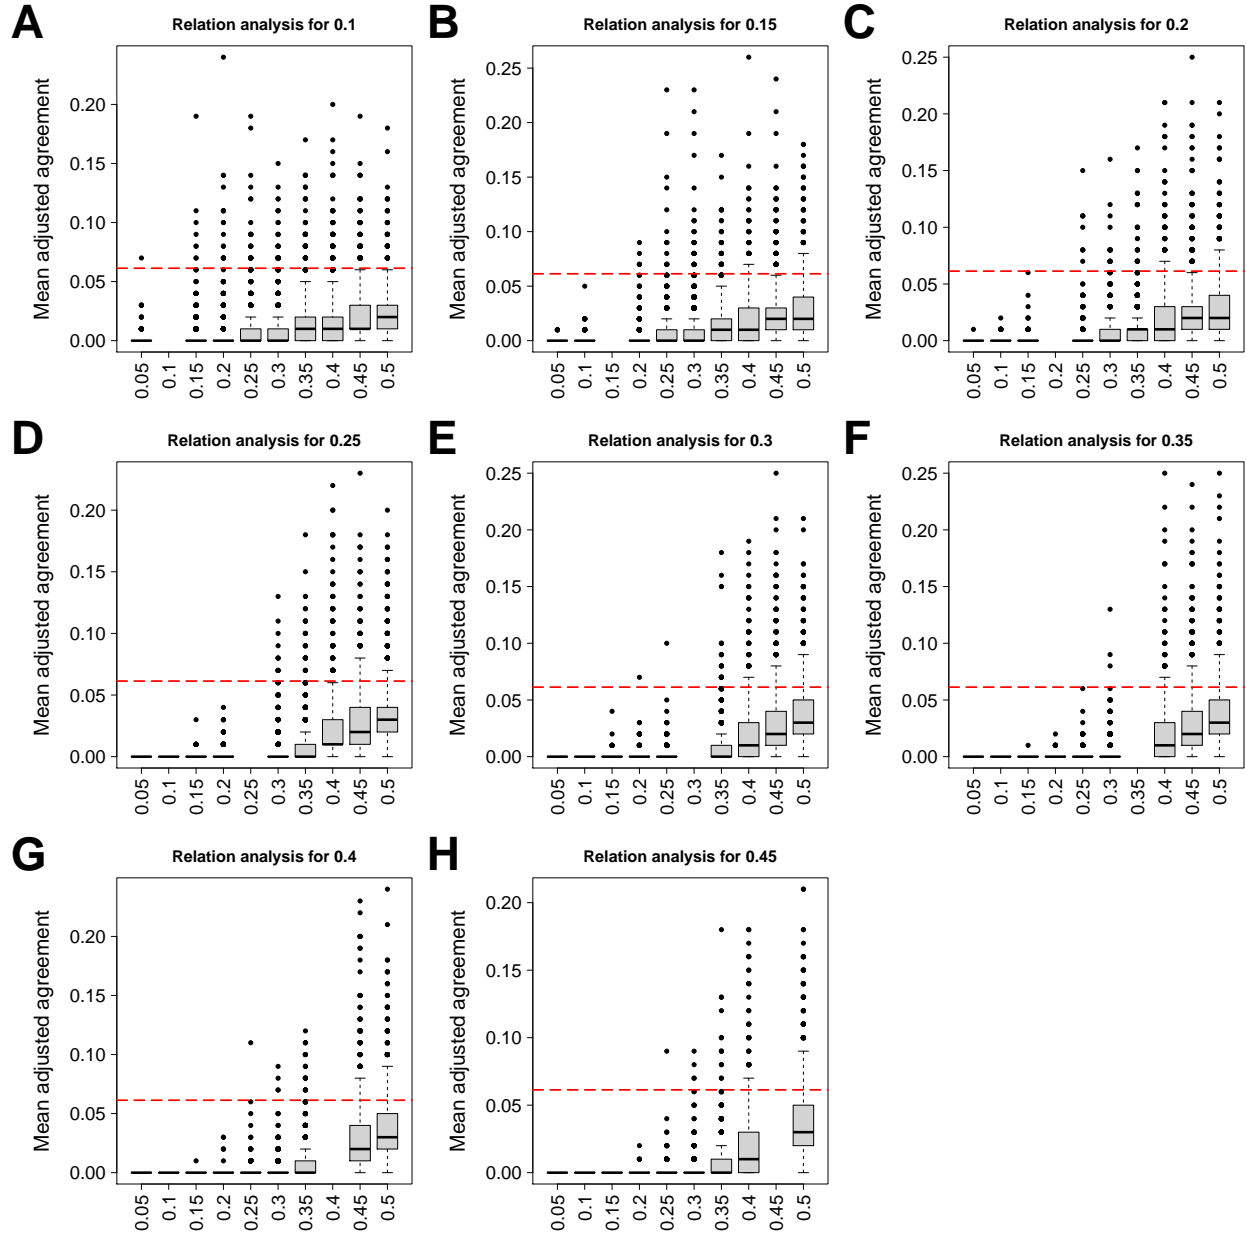

Figure S 3: Null Scenario B (classification): Relation analysis based on mean adjusted agreement for the variables with minor allele frequencies of 0.1 to 0.45. The dashed line shows the threshold for the selection of related variables. The relations of the other variables are shown in Figure 2.

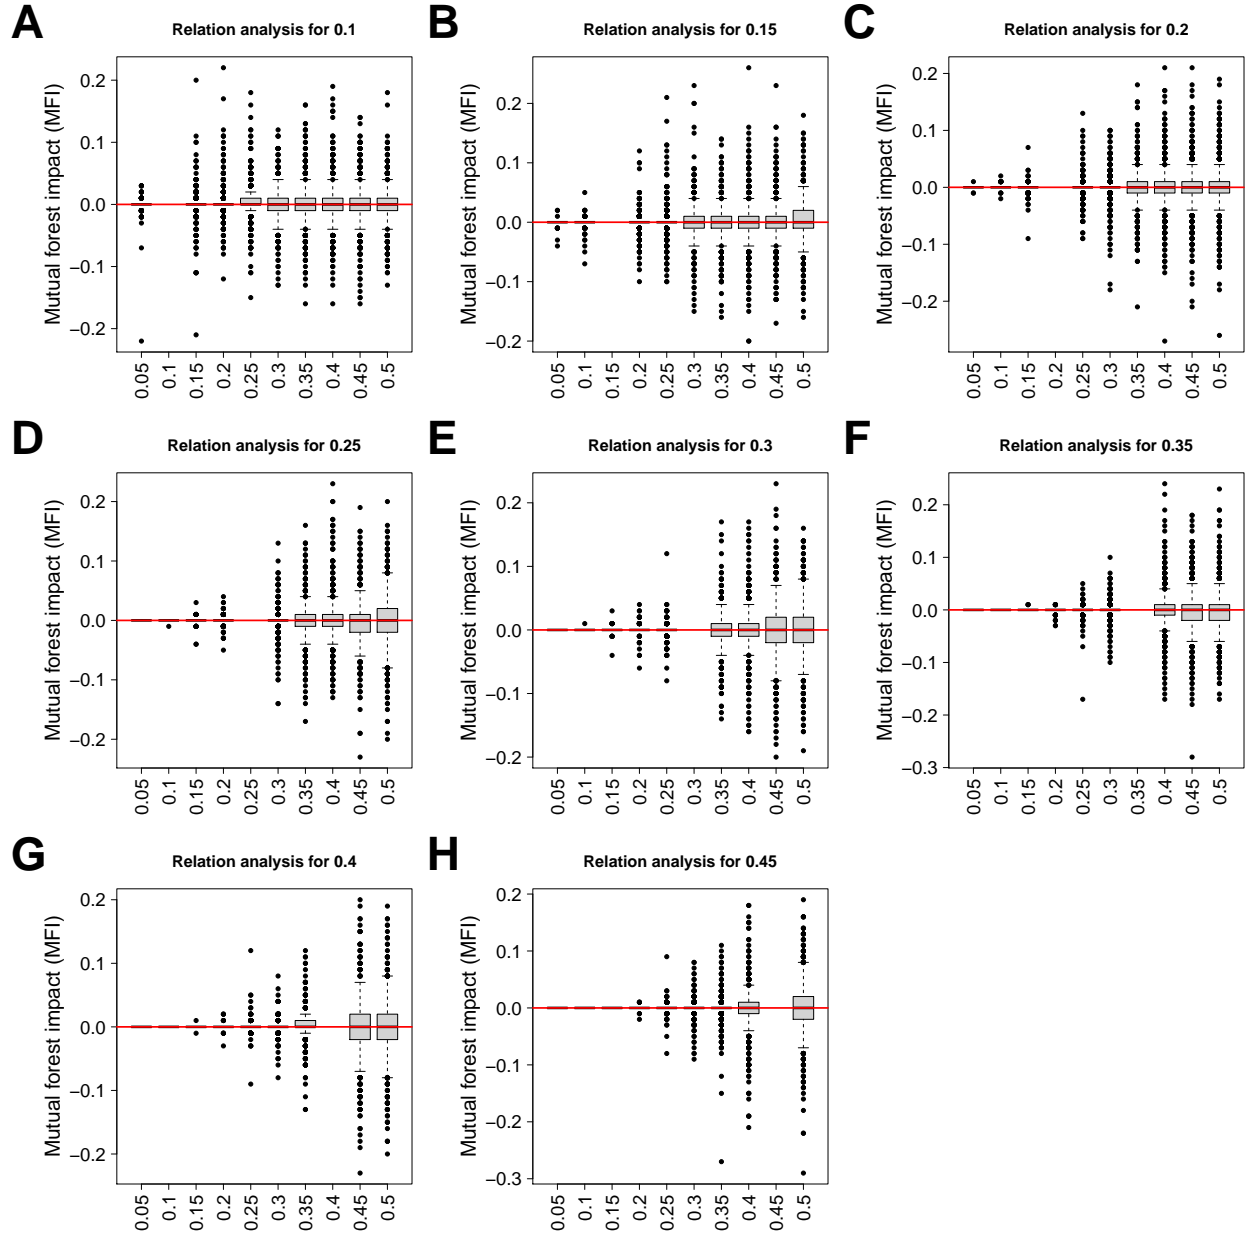

Figure S 4: Null Scenario B (classification): Relation analysis based on MFI for the variables with minor allele frequencies of 0.1 to 0.45. The dashed line shows a relation value of 0. The relations of the other variables are shown in Figure 2.

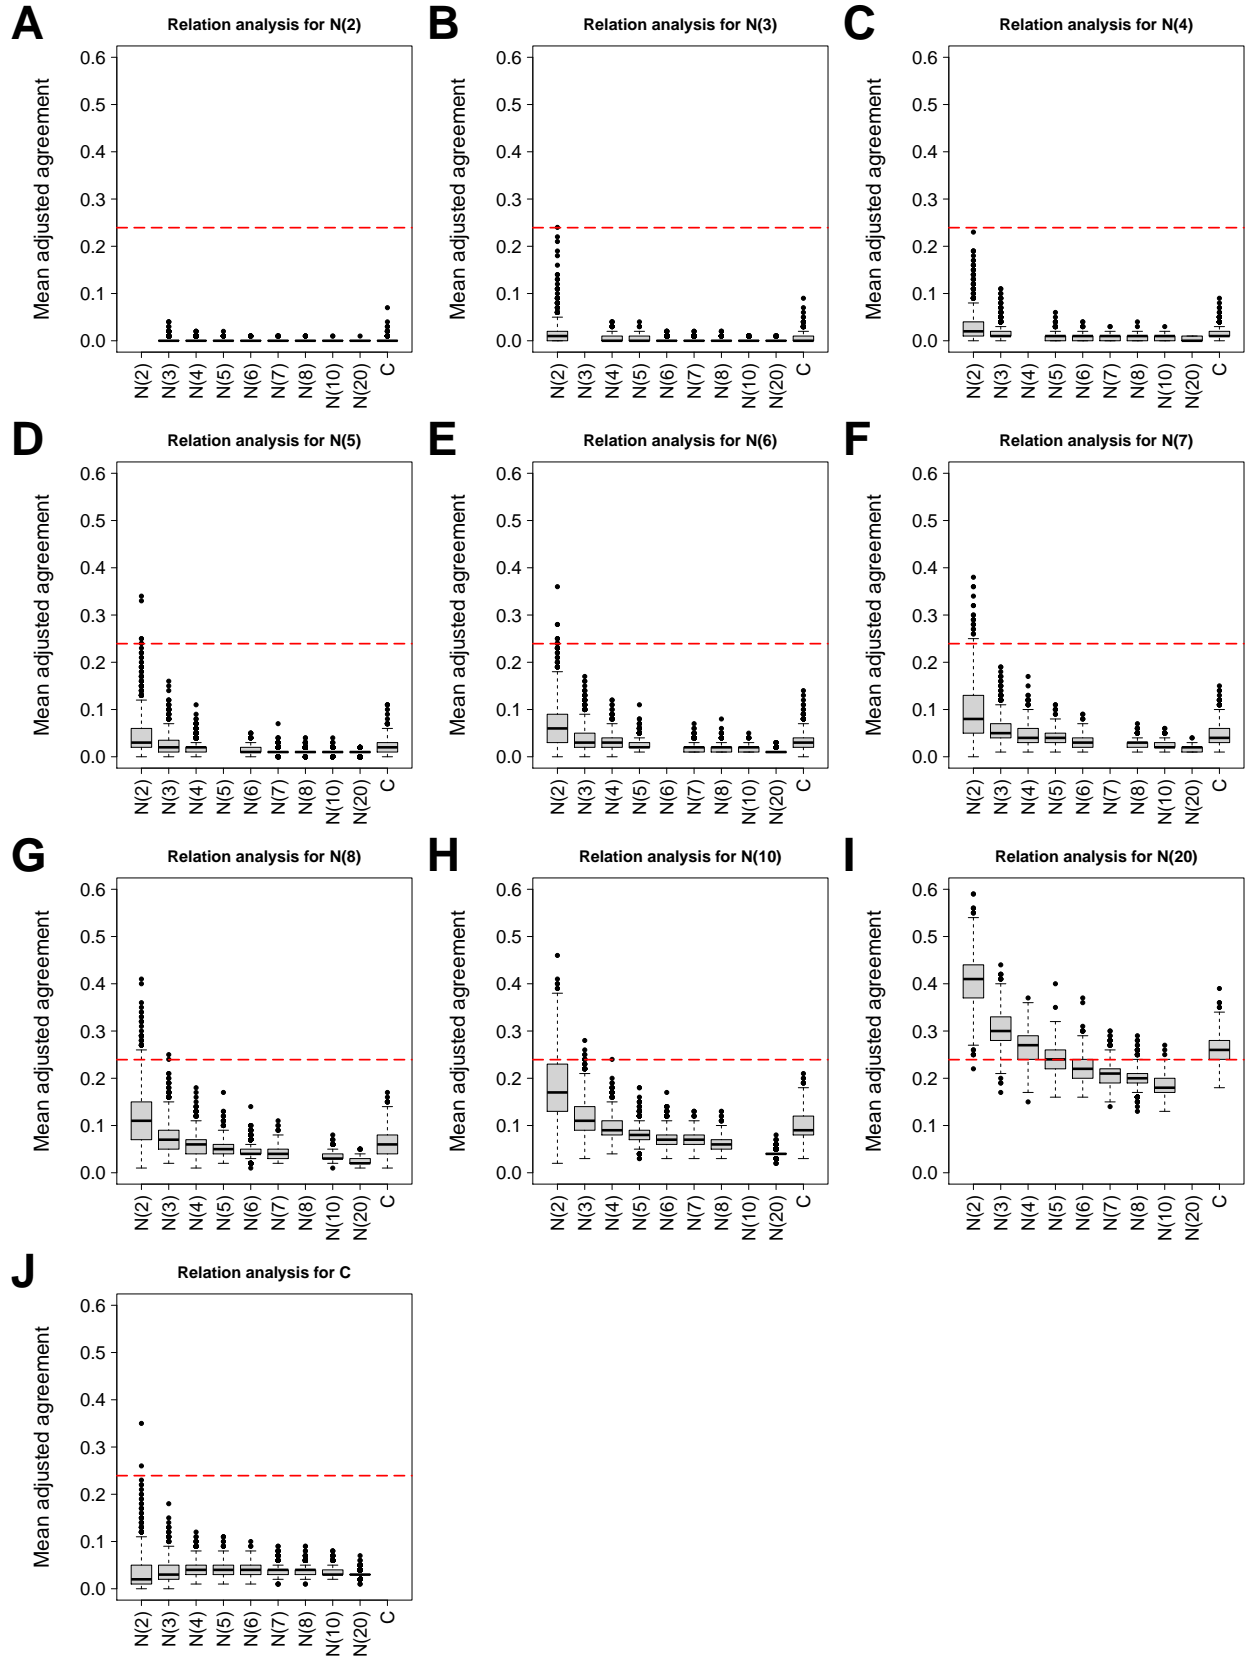

Figure S 5: Null Scenario A (regression): Relation analysis based on mean adjusted agreement for the nominal variables (A-I) and the continuous variable (J). The dashed line shows the threshold for the selection of related variables.

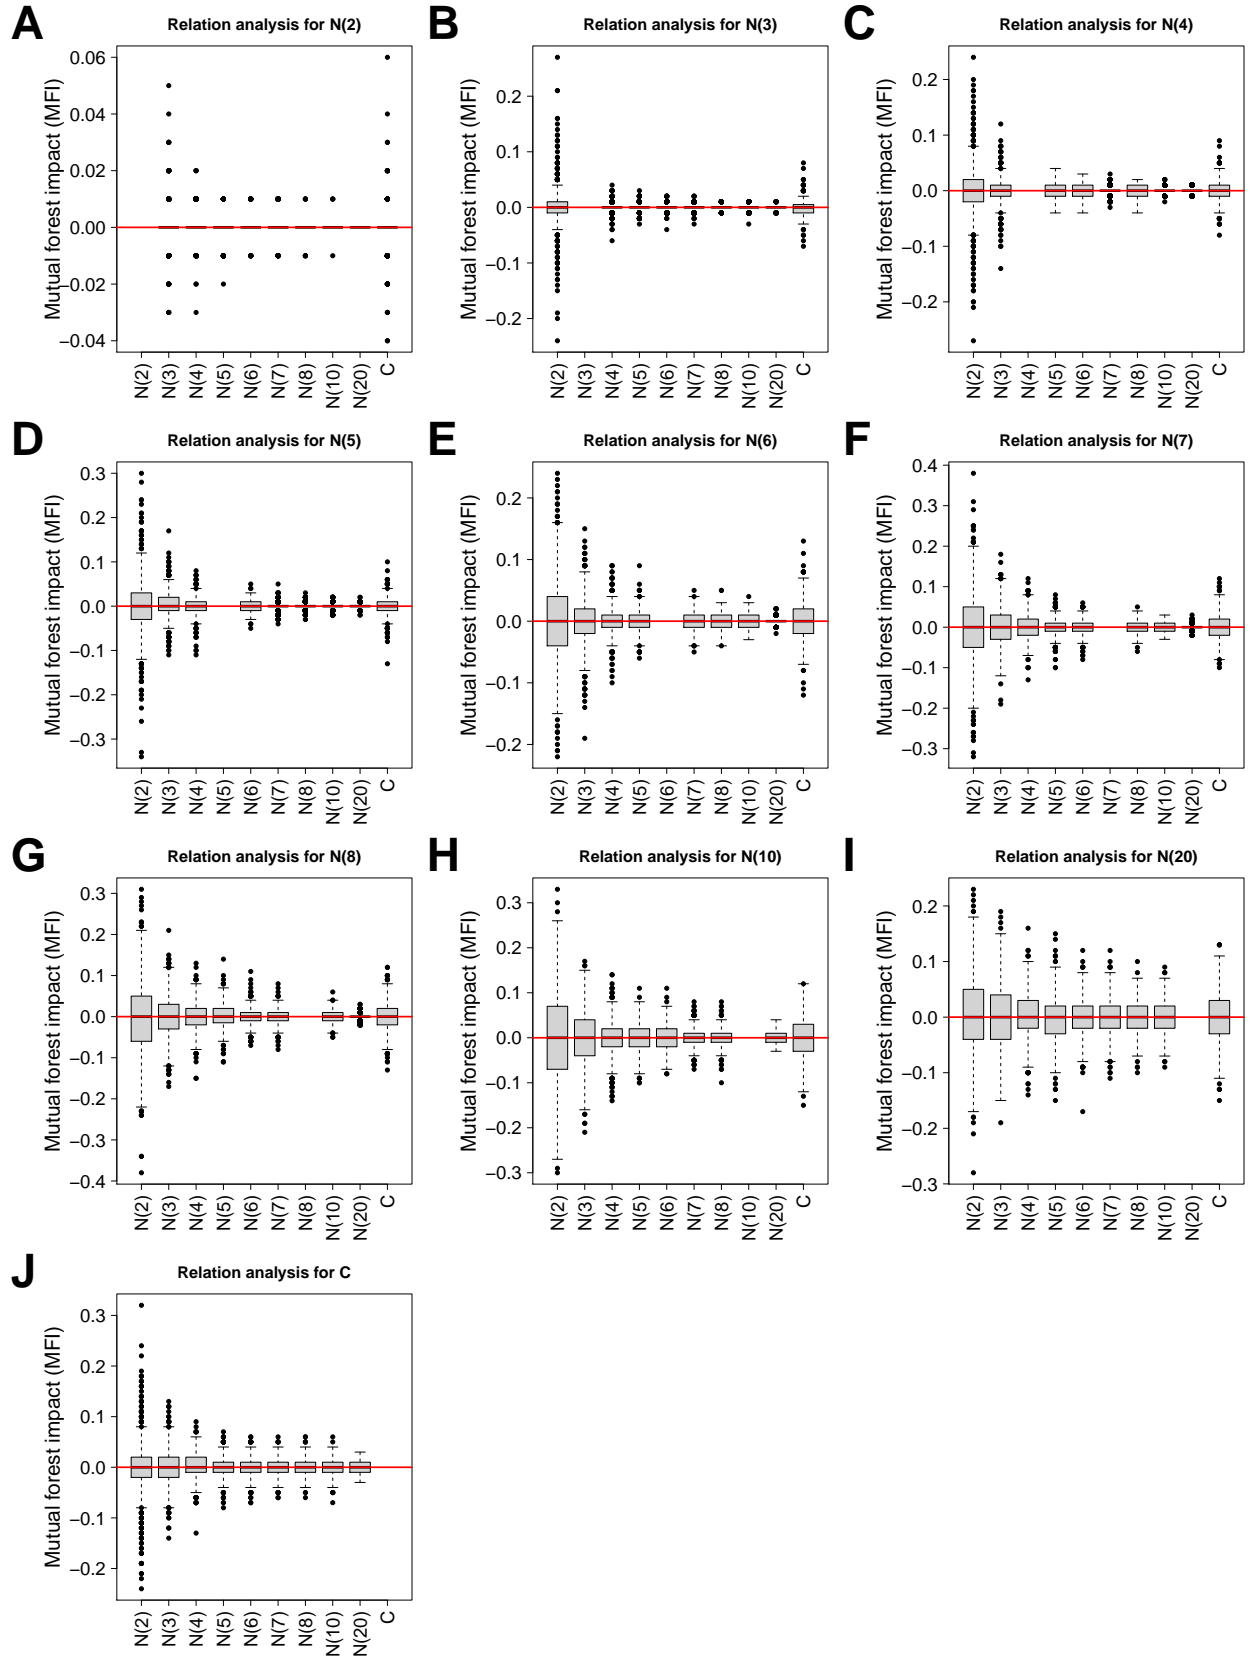

Figure S 6: Null Scenario A (regression): Relation analysis based on MFI for the nominal variables (A-I) and the continuous variable (J). The dashed line shows a relation value of 0.

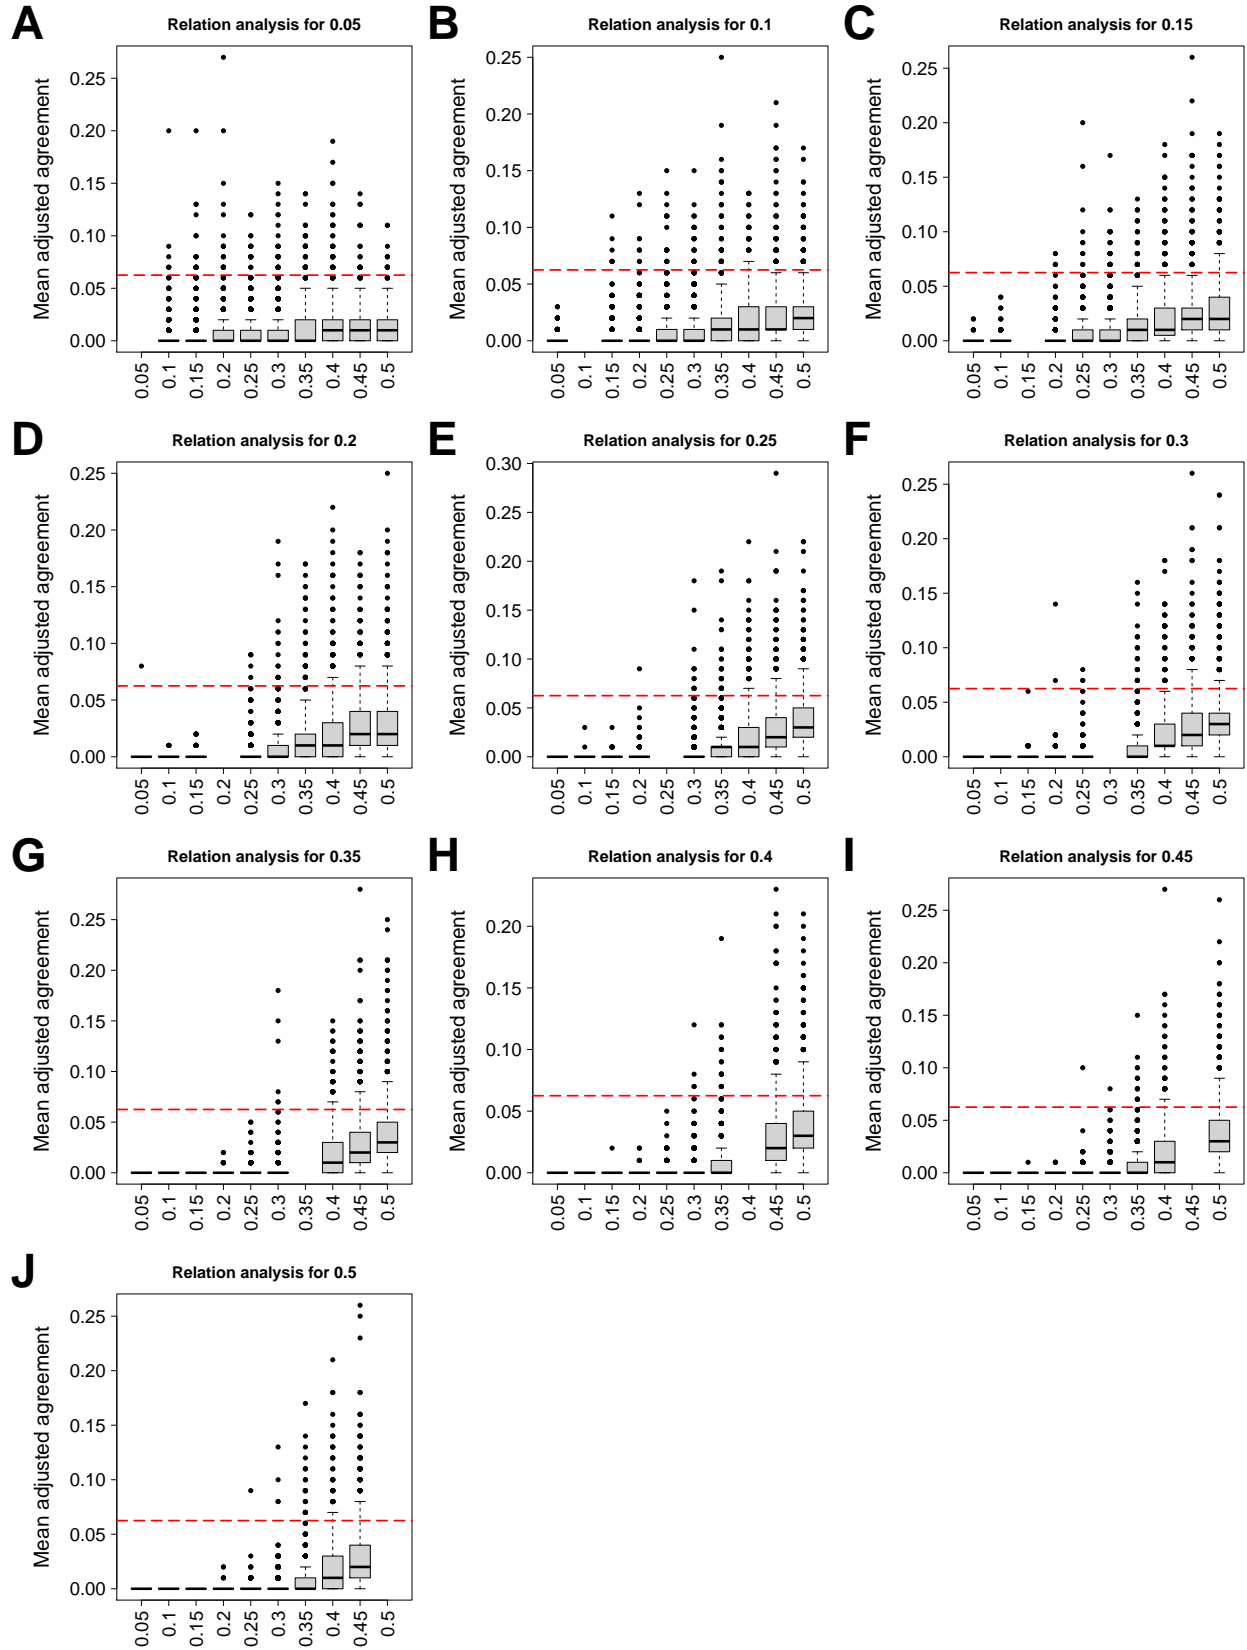

Figure S 7: Null Scenario B (regression): Relation analysis based on mean adjusted agreement for the variables with different minor allele frequencies. The dashed line shows the threshold for the selection of related variables.

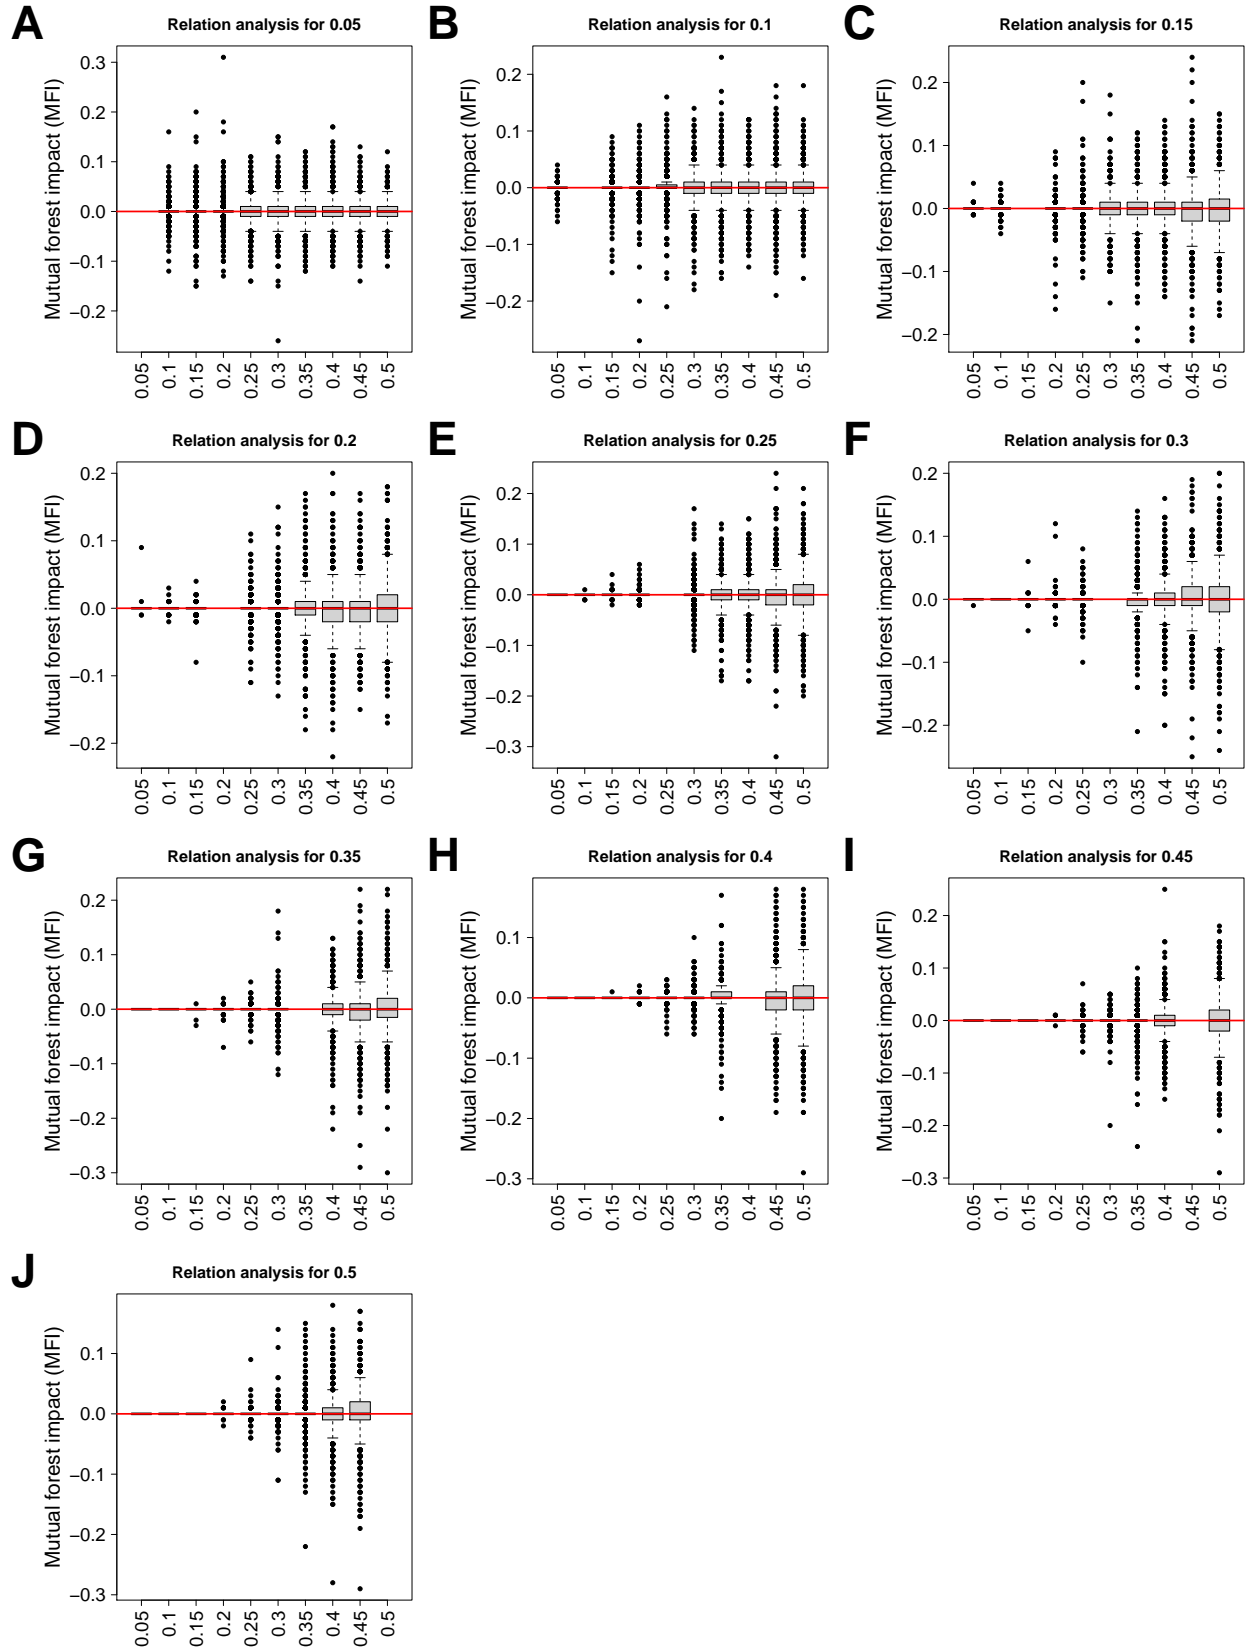

Figure S 8: Null Scenario B (regression): Relation analysis based on MFI for the variables with different minor allele frequencies. The dashed line shows a relation value of 0.

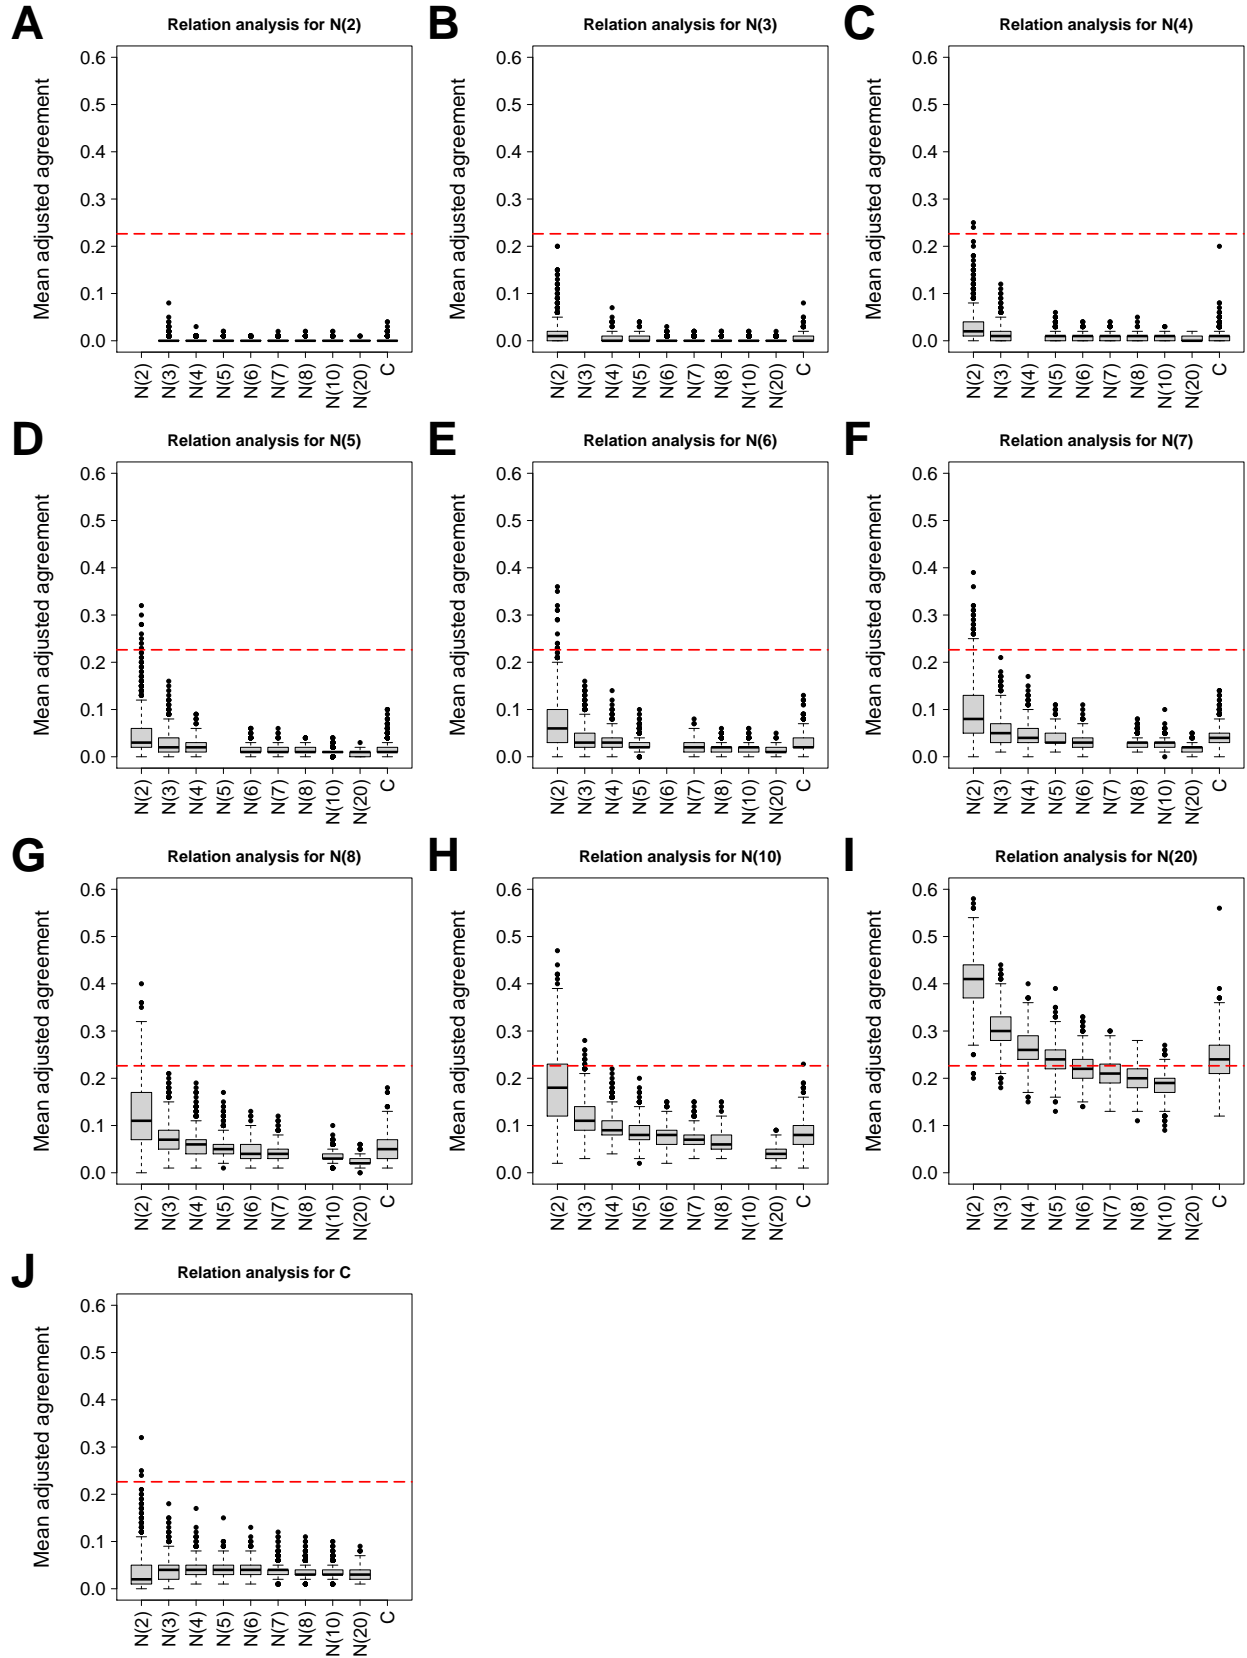

Figure S 9: Null Scenario A (survival): Relation analysis based on mean adjusted agreement for the nominal variables (A-I) and the continuous variable (J). The dashed line shows the threshold for the selection of related variables.

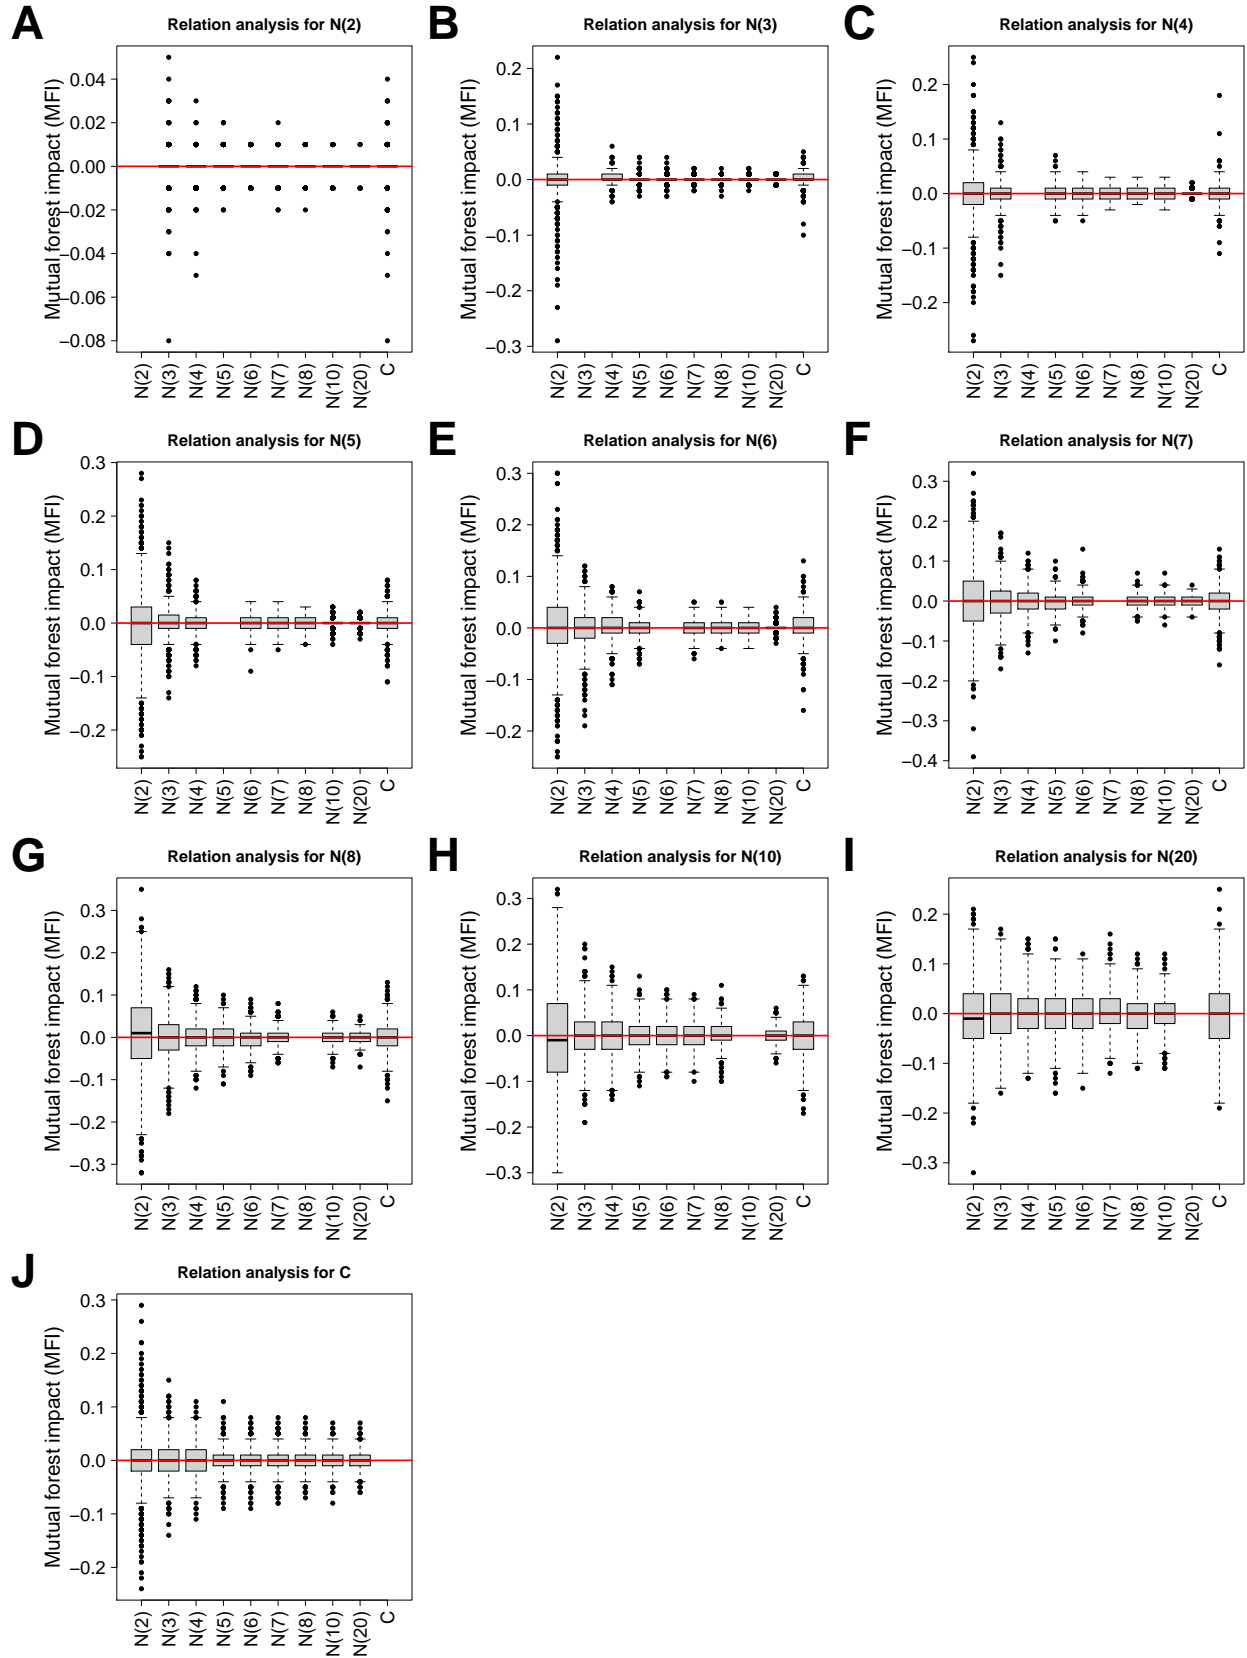

Figure S 10: Null Scenario A (survival): Relation analysis based on MFI for the nominal variables (A-I) and the continuous variable (J). The dashed line shows a relation value of 0.

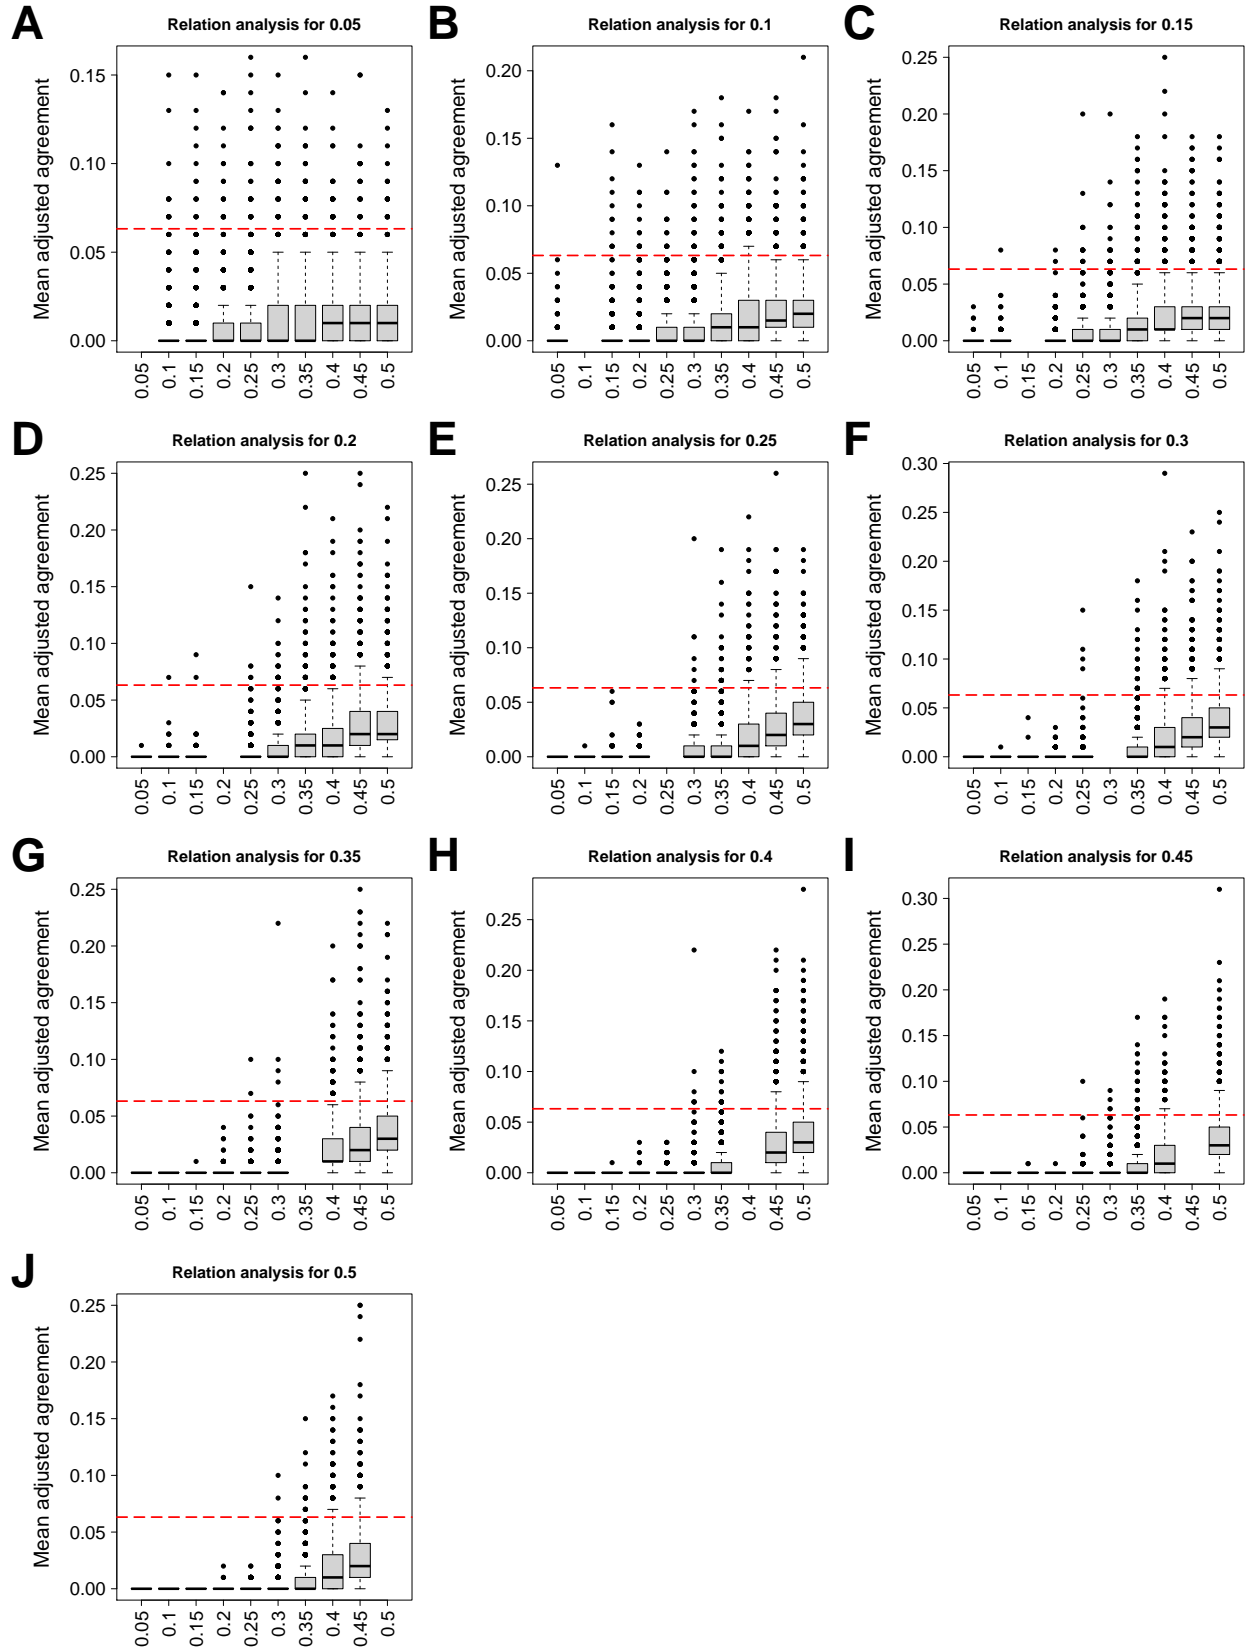

Figure S 11: Null Scenario B (survival): Relation analysis based on mean adjusted agreement for the variables with different minor allele frequencies. The dashed line shows the threshold for the selection of related variables.

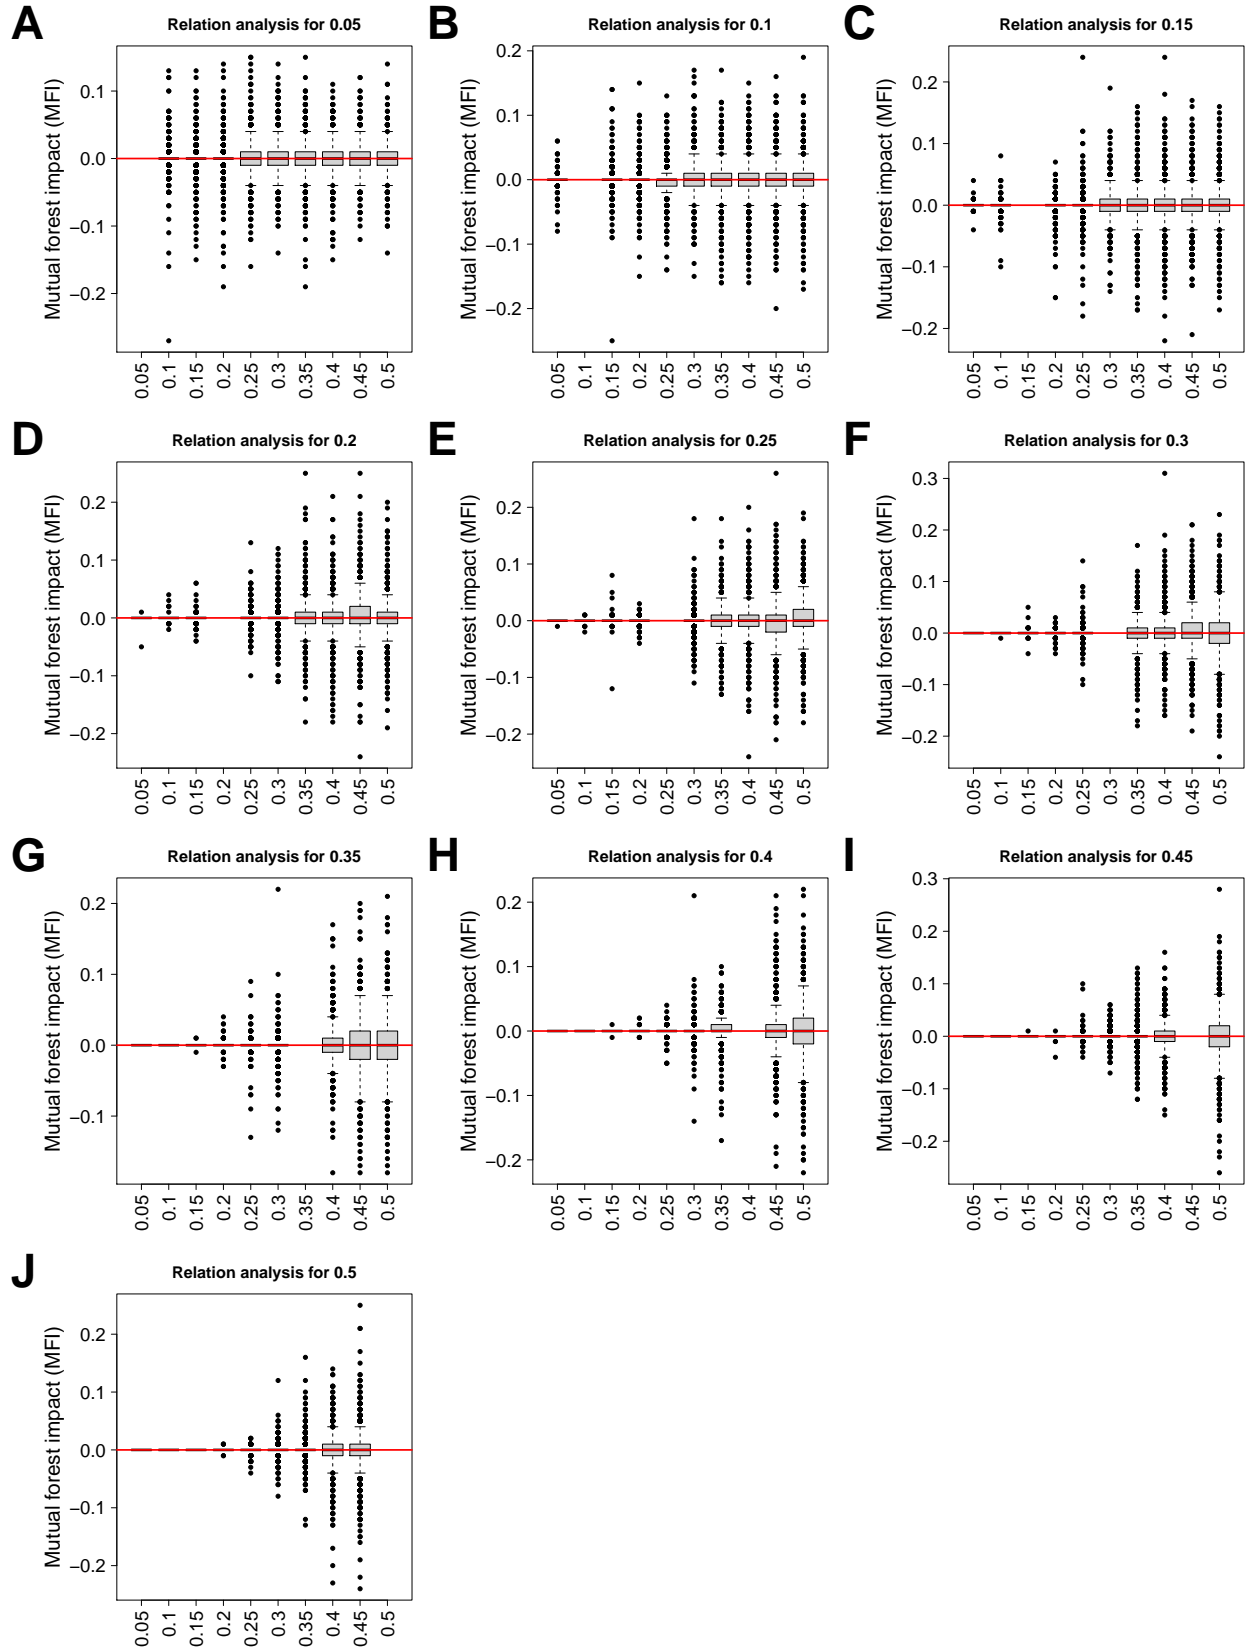

Figure S 12: Null Scenario B (survival): Relation analysis based on MFI for the variables with different minor allele frequencies. The dashed line shows a relation value of 0.

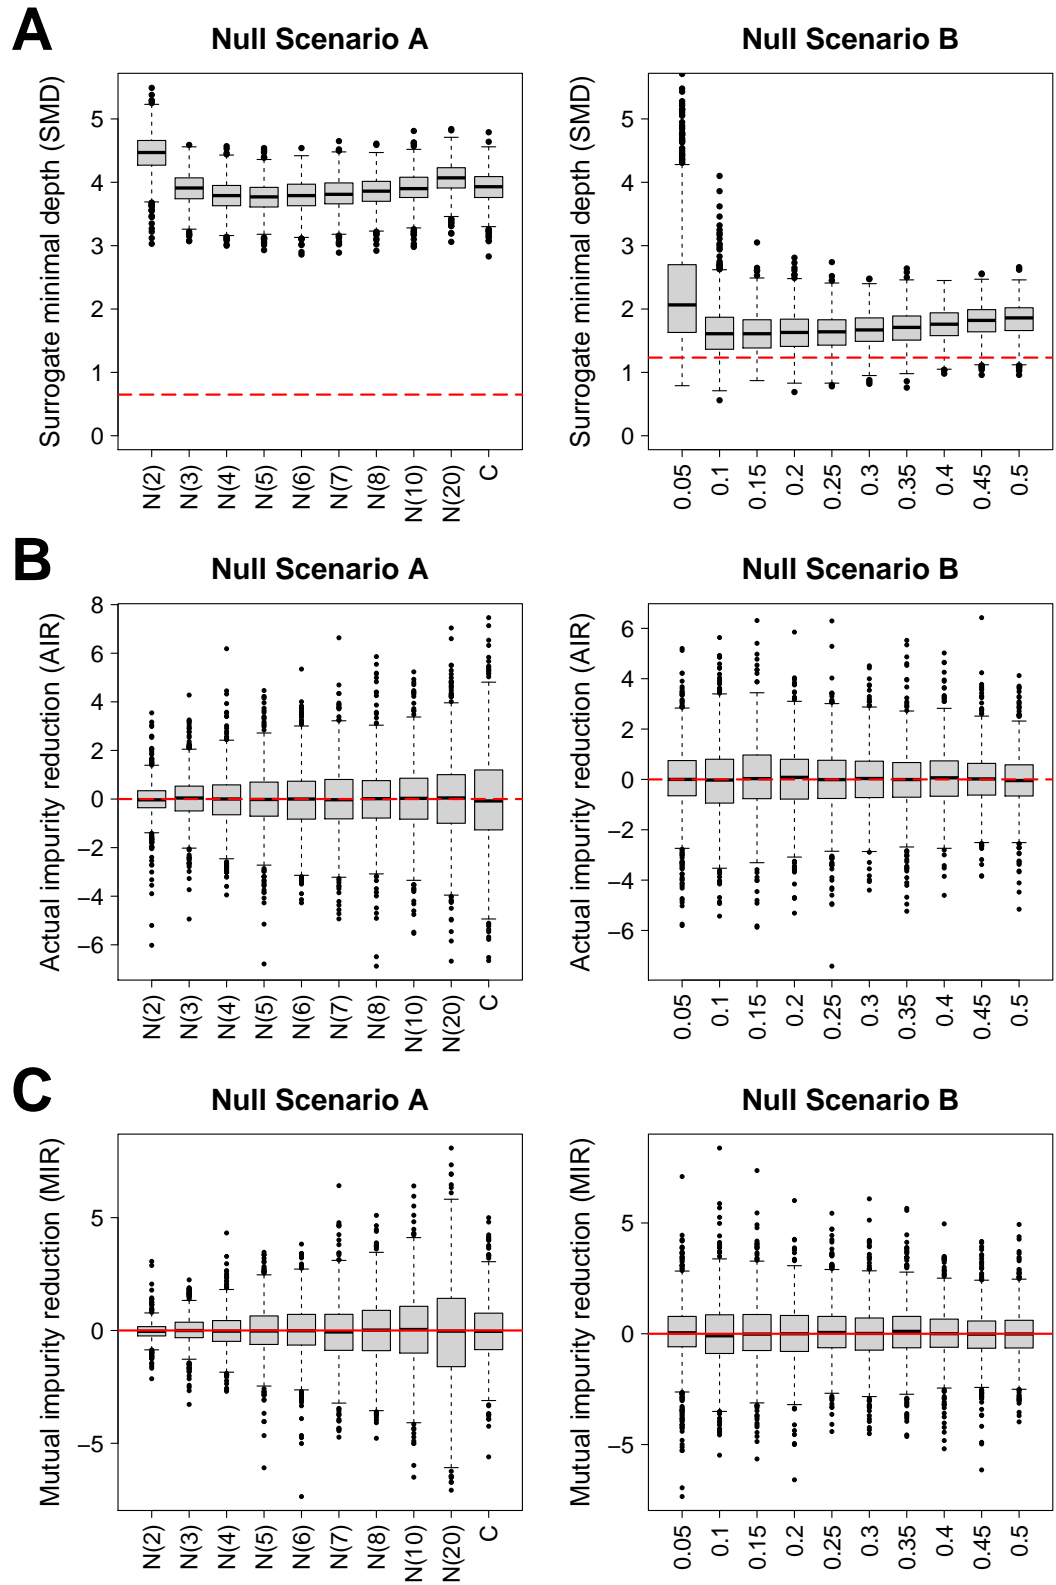

Figure S 13: Variable importances for Null scenarios (regression): Results of SMD (A), AIR (B), and MIR (C) in Null Scenario A (left) and B (right). The dashed line shows the threshold for the feature selection and an importance value of 0 for SMD ( $t=5$ ) and AIR and MIR, respectively.

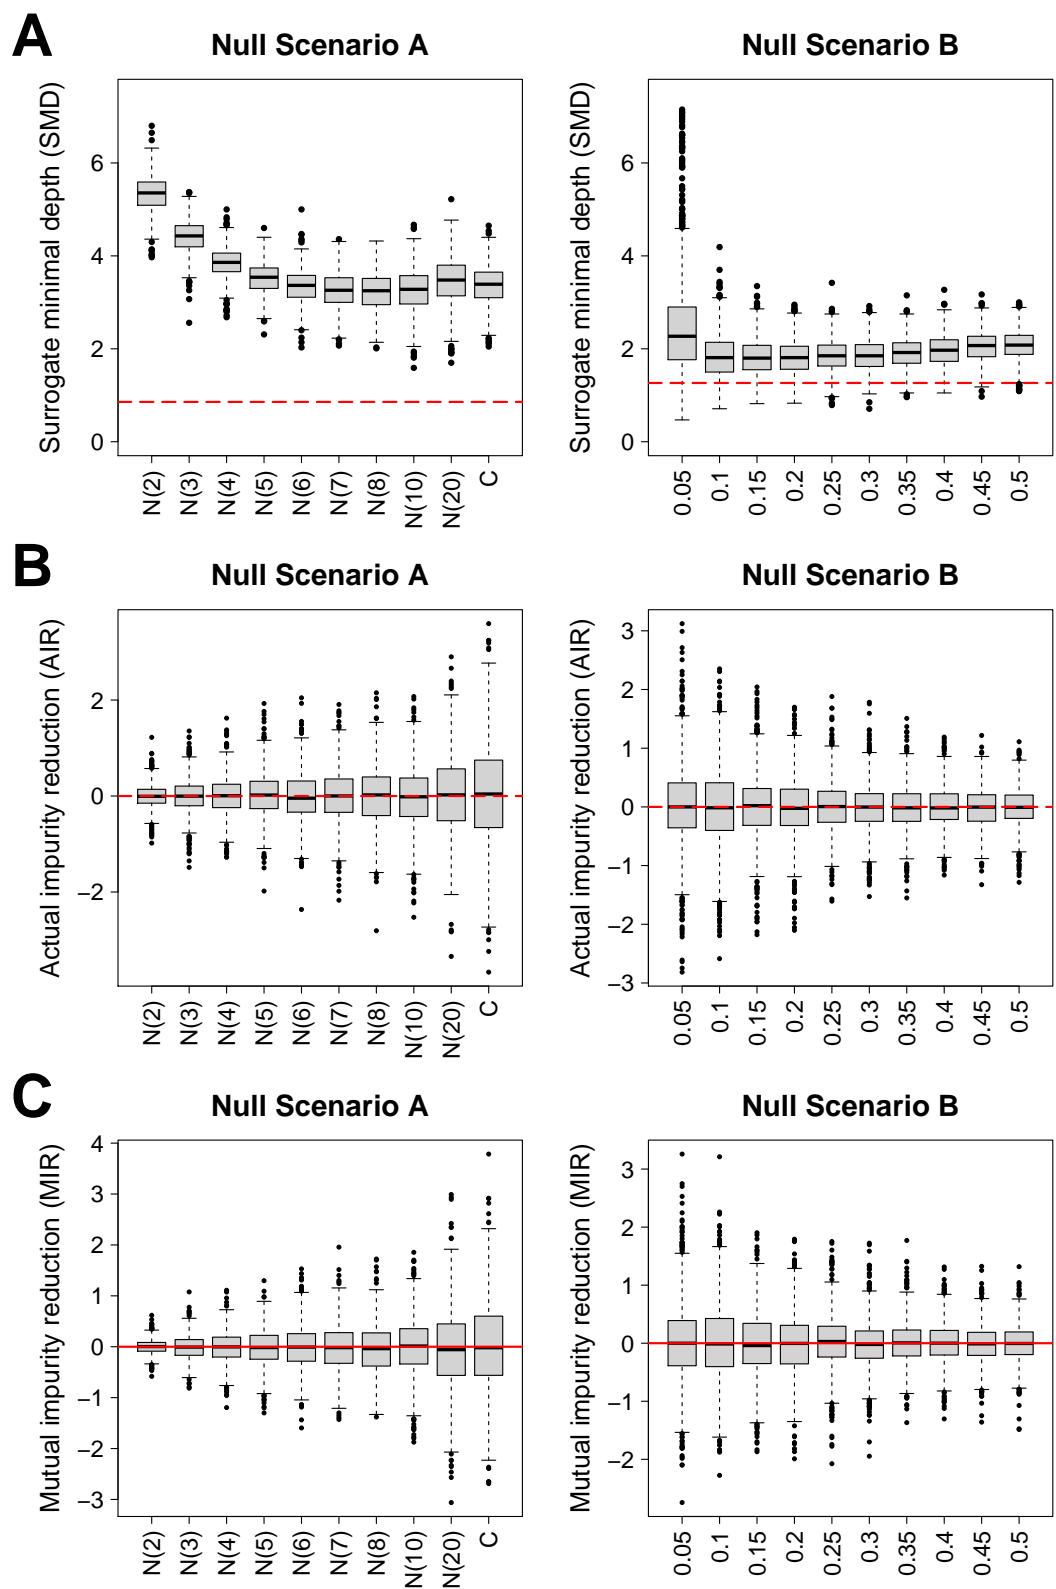

Figure S 14: Variable importances for Null scenarios (survival): Results of SMD (A), AIR (B), and MIR (C) in Null Scenario A (left) and B (right). The dashed line shows the threshold for the feature selection and an importance value of 0 for SMD ( $t=5$ ) and AIR and MIR, respectively.

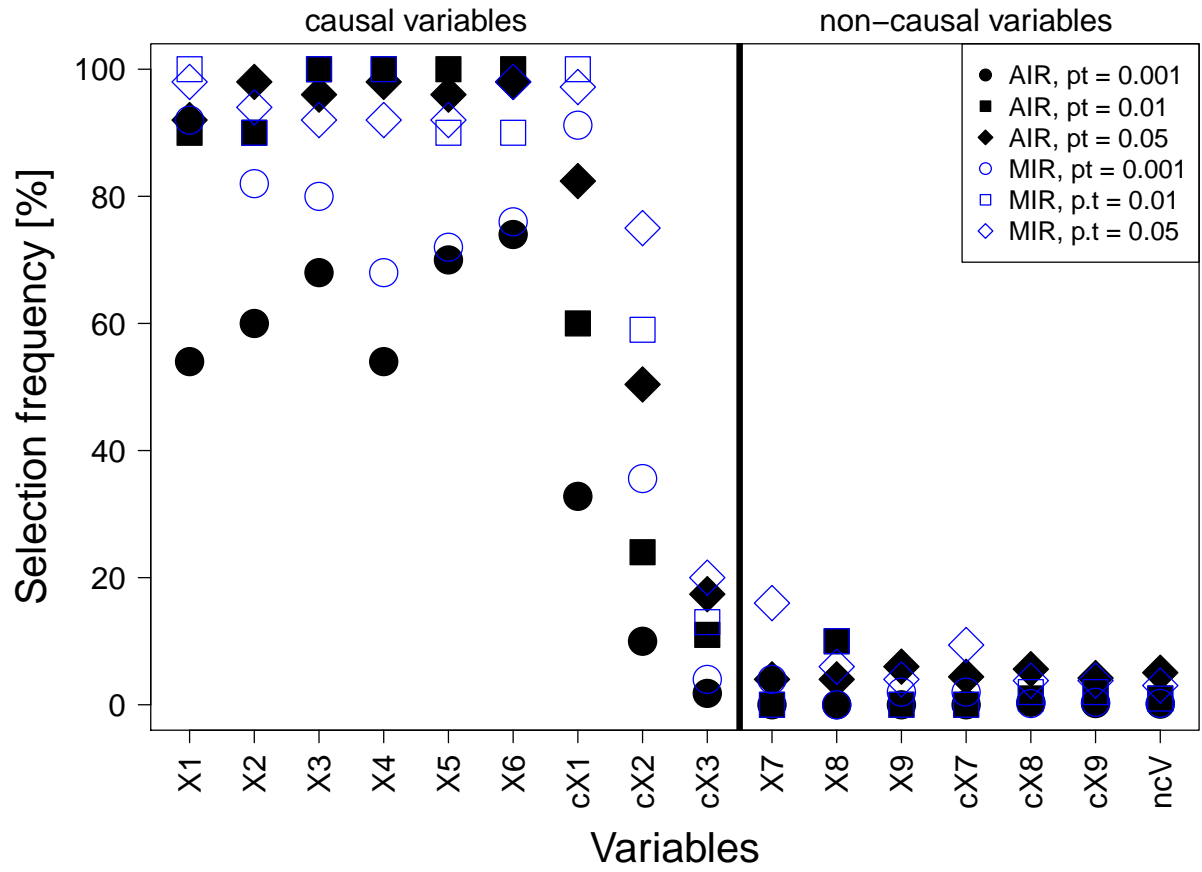

Figure S 15: Results of the correlation study utilizing different numbers p-value thresholds for MIR and AIR. For the basic variables, ( $X_1 - X_9$ ) the selection frequencies are averaged across all 50 replicates, whereas for the six groups of correlated variables, ( $cX_1 - cX_3$  and  $cX_7 - cX_9$ ) as well as the non-causal variables (ncVs) the average frequencies across all replicates and variables in the respective group are shown.

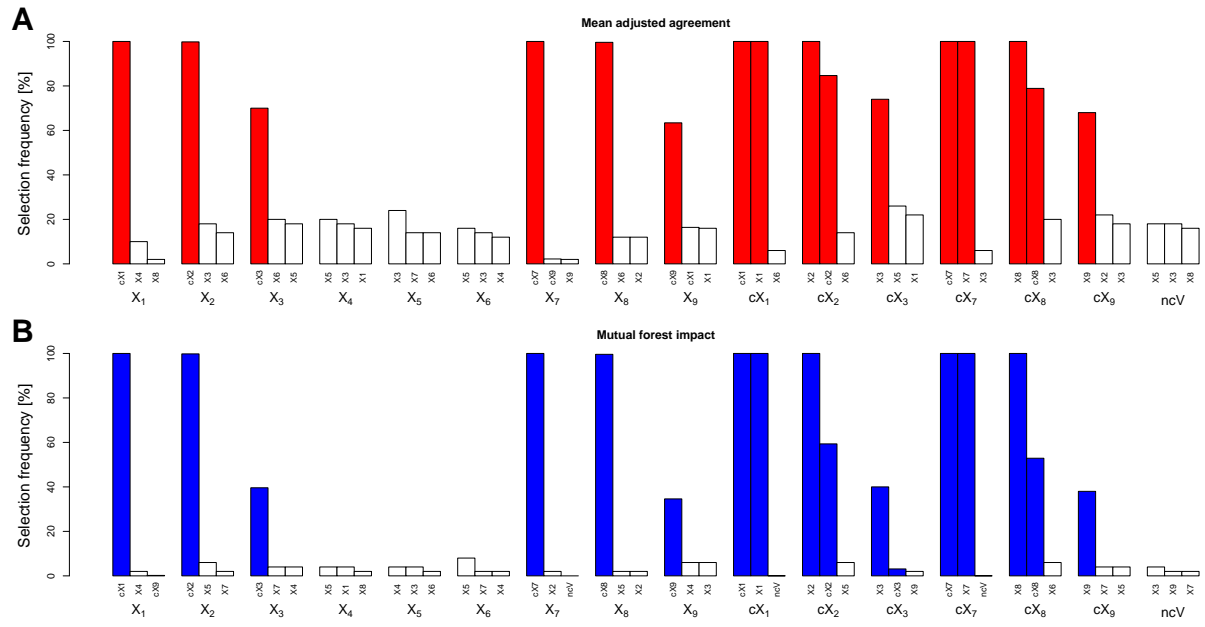

Figure S 16: Variable relation selection frequencies based on mean adjusted agreement (A) and mutual forest impact (B) utilizing a t-value of 5 and a p-value threshold of 0.01, respectively. Results for the basic variables ( $X_1 - X_9$ ) and the first variable of each group of variables ( $cX_1, cX_2, cX_3, cX_6, cX_7, cX_9$ ) are shown. For each variable, the three most often selected variables are shown and the different groups were summarized in one plot. The bars of the correlated variables are colored in red and blue for SMD and MIR, respectively.

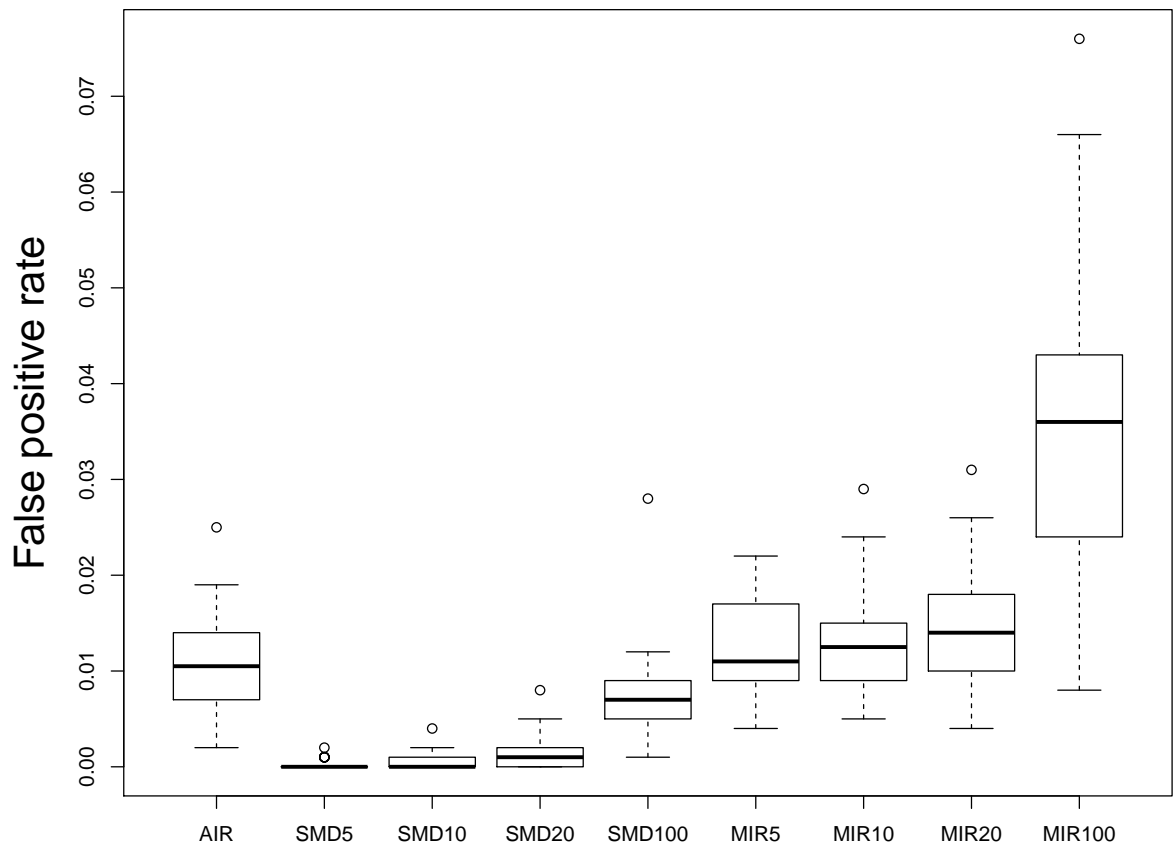

Figure S 17: Results of the null scenario. AIR and MIR were applied with a p-value threshold of 0.01 and SMD and MIR with different numbers of surrogates specified below the respective boxplot
